# Supplementary material for: MURA: Large Dataset for Abnormality Detection in Musculoskeletal Radiographs
Source: arXiv:1712.06957 source file (2018-05-22)
Supplement: Supplementary file 1 [file appendix.tex]

\setcounter{table}{0}

\section{Appendix}

\input{tables/distribution}
